# Supplementary material for: From Clustering to Cluster Explanations via Neural Networks
Source: arXiv:1906.07633 source file (2021-12-16)
Supplement: Supplementary file 1 [file supplement.tex]

% \pdfoutput=1

\documentclass[journal,onecolumn]{IEEEtran}
\oddsidemargin=0.25in
\topmargin=-0.25in
\textwidth=6in
\textheight=9in

\usepackage{amsmath,amssymb,amsthm,mathtools}
\usepackage{graphicx,dblfloatfix}
\usepackage{graphbox}
\usepackage{bbm}
\usepackage{cite,xcolor}
\usepackage{booktabs}
\usepackage{url}

\newtheorem{lemma}{Lemma}
\DeclareMathOperator*{\LME}{LME}

\newcounter{countrevision}
\makeatletter
\@addtoreset{countrevision}{section}
\makeatother

\newcounter{countnetwork}
\usepackage{tikz}
\usepackage[framemethod=tikz]{mdframed}
\newenvironment{boxnetwork}[1][]{%
\mdfsetup{% 
	frametitle={%
		\tikz[baseline=(current bounding box.east),outer sep=0pt] \node[anchor=east,rounded corners=3pt,fill=gray!30]
		{\strut\,#1\,};}%
}% 
\mdfsetup{%
	skipabove=7mm,skipbelow=4mm,%
	leftmargin=2.5cm,rightmargin=2.5cm,
	backgroundcolor=gray!10,
	innertopmargin=-10pt,innerbottommargin=5pt,
	innerleftmargin=2pt,innerrightmargin=2pt,
	linecolor=gray!30,%
	linewidth=1pt,topline=true,%
	roundcorner=3pt,
	frametitlealignment={\hspace*{0.02\linewidth}},
	frametitleaboveskip=-10pt,
	frametitlefont=\normalfont\bf}\refstepcounter{countnetwork}\begin{mdframed}[nobreak=true]\relax%
}{\end{mdframed}}

\newcommand{\centroid}{\boldsymbol{\mu}}
\newcommand{\sv}{\boldsymbol{u}}
\newcommand{\x}{\boldsymbol{x}}
\newcommand{\ba}{\boldsymbol{a}}

\newcommand{\w}{\boldsymbol{w}}

\newcommand{\kmeans}{k-means}

\allowdisplaybreaks

\begin{document}

\title{
From Clustering to Cluster Explanations\\via Neural Networks\\{\large \sc \sffamily (Supplementary Material)}
}

\author{Jacob Kauffmann, Malte Esders, Lukas Ruff, Gr\'egoire Montavon,\\ Wojciech Samek, Klaus-Robert M\"uller}

\maketitle

\noindent
This document contains supplementary material supporting the results and experiments from the main paper. Appendices \ref{appendix:neuralization}--\ref{appendix:neuralization-soft} contain proofs and justifications for some of the non-trivial steps taken in Sections II--IV of the main paper to neuralize the k-means models. Appendix \ref{appendix:training} describes the modified training procedure used for producing the kernel k-means models of Sections VI-A and VII of the main paper. Appendices \ref{appendix:datasets}--\ref{appendix:vgg16} give additional information, evaluations, and results, for the experiments of Sections VI-C and VII of the main paper.

\appendices

\section{Neuralization of \kmeans{}}
\label{appendix:neuralization}

We recall that the decision function implemented by \kmeans{} can be expressed as:
\input{equations/decision}
i.e.\ one assigns a given data point $\x$ to the cluster $c$ if every other cluster $k \neq c$ has higher distance between the data point and the cluster centroid.

\input{propositions/neuralization}

\begin{proof}
We first note that the decision function of Eq.\ \eqref{eq:decision} can be rewritten more compactly by testing only for the nearest cluster competitor, i.e.\
\begin{align}
\|\x-\centroid_c\|^2 < \min_{k \neq c} \|\x-\centroid_k\|^2.
\label{eq:decision-min}
\end{align}
If this holds, the same necessarily holds for all remaining cluster competitors. We now rewrite the function $f_c(\x)$ computed at the output of the neural network model in a way that let appear distances:
\begin{align*}
f_c(\x) &= \min_{k \neq c} \{h_k\}\\
    &= \min_{k\neq c}\lbrace \boldsymbol{w}_k^\top\x + b_k\rbrace\\
    &= \min_{k\neq c}\lbrace -2\x^\top\centroid_k + \|\centroid_k\|^2 + 2\x^\top\centroid_c - \|\centroid_c\|^2\rbrace\\
    &= \min_{k\neq c}\lbrace\|\x - \centroid_k\|^2 - \|\x - \centroid_c\|^2\rbrace\\
    &= -\|\x - \centroid_c\|^2 + \min_{k\neq c}\lbrace\|\x - \centroid_k\|^2\rbrace
\end{align*}
It can now be seen easily that the predicate $f_c(\x)>0$ is equivalent to Eq.\ \eqref{eq:decision-min}.
\end{proof}

\section{Shapley Value Reductions}
\label{appendix:shapley}

Let $\x \in \mathbb{R}^d$ be our data point. Let $\mathcal{I}$ denote a collection of input features, and $\x_\mathcal{I}$ denote the data point $\x$ where values for features $i \notin \mathcal{I}$ have been replaced by the corresponding values of some reference data point $\widetilde{\x}$. In particular, denoting by $\Omega$ the set of all $d$ features and by $\varnothing$ the empty set, we have $\x_\Omega = \x$ and $\x_{\varnothing} = \widetilde{\x}$. We consider a function $f:\mathbb{R}^d \to \mathbb{R}$ mapping the data points to real-valued scores. In this context, the Shapley Value provides a way of attributing this score to the individual input features via the formula
\begin{align}
R_i = \sum_{\mathcal{I} \subseteq \Omega \setminus \{i\}} \alpha_{\mathcal{I}} \cdot \big[f(\x_{\mathcal{I} \cup \{i\}}) - f(\x_\mathcal{I})\big],
\end{align}
where $\alpha_{\mathcal{I}} = |\mathcal{I}|! \cdot (|\Omega|-|\mathcal{I}|-1)! / |\Omega|!$ is a weighting coefficient satisfying $\sum_{\mathcal{I} \subseteq \Omega \setminus \{i\}} \alpha_{\mathcal{I}} = 1$. We first present two (known) intermediate results that we can use to prove Propositions \ref{proposition:shapley-hidden} and \ref{proposition:shapley-twoclusters} of the main paper.

\begin{lemma}
Let $\x \in \mathbb{R}_+^d$. The Shapley Value of the function $f(\x) = \min\{x_1,\dots,x_d\}$ with replacement value $\widetilde{\x} = \boldsymbol{0}$ is $R_i = f(\x) / d$.
\label{lemma:min}
\end{lemma}
\begin{proof}
\begin{align}
R_i &= \sum_{\mathcal{I} \subseteq \Omega \setminus \{i\}} \alpha_{\mathcal{I}} \cdot \big[f(\x_{\mathcal{I} \cup \{i\}}) - f(\x_\mathcal{I})\big] \label{eq:shapley-min1}\\
&= \sum_{\mathcal{I} \subseteq \Omega \setminus \{i\}} \alpha_{\mathcal{I}} \cdot f(\x_{\mathcal{I} \cup \{i\}}) \label{eq:shapley-min2}\\
&= \alpha_{\Omega \setminus \{i\}} \cdot f(\x_{\Omega}) \label{eq:shapley-min3}\\
&= \frac1d \cdot f(\x) \label{eq:shapley-min4}
\end{align}
From \eqref{eq:shapley-min1} to \eqref{eq:shapley-min2}, we have made use of the fact that setting one of the inputs to zero in the $\min$ function suffices to make the output of that function zero. Specifically, the rightmost term, which never includes feature $i$ is therefore always zero and can be dropped. From \eqref{eq:shapley-min2} to \eqref{eq:shapley-min3}, we have observed that only one element in the sum has an associated function value that is non-zero, specifically, the one for which all features are included. From \eqref{eq:shapley-min3} to \eqref{eq:shapley-min4}, we simply replace the coefficient $\alpha$ by its numerical value, and observe that $\x_\Omega$ and $\x$ denote the same quantity.
\end{proof}

\begin{lemma}
Let $\x \in \mathbb{R}^d$. The Shapley value of a linear model $f(\x) = \w^\top \x + b$ when choosing replacement value $\widetilde{\x}$ is $R_i = w_i \cdot (x_i - \widetilde{x}_i)$.
\label{lemma:linear}
\end{lemma}
\begin{proof}
\begin{align}
R_i &= \sum_{\mathcal{I} \subseteq \Omega \setminus \{i\}} \alpha_\mathcal{I} \cdot \big[f(\x_{\mathcal{I} \cup \{i\}}) - f(\x_\mathcal{I})\big]\\
&= \sum_{\mathcal{I} \subseteq \Omega \setminus \{i\}} \alpha_\mathcal{I} \cdot (w_i x_i - w_i \widetilde{x}_i)\\
&= w_i \cdot (x_i - \widetilde{x}_i) \cdot \!\!\! \underbrace{\sum_{\mathcal{I} \subseteq \Omega \setminus \{i\}} \alpha_\mathcal{I}}_{1}
\end{align}
\end{proof}

\subsection{Attribution on Intermediate Layer}

We recall that in the main paper, we have proposed to perform redistribution in the second layer of neuralized k-means using the rule
\input{equations/rule-mintakemost}
where the latter interpolates between min-take-all redistribution when $\beta \to \infty$ and uniform redistribution when $\beta = 0$.
\input{propositions/shapley-hidden}
\begin{proof}
This is a direct consequence of Lemma \ref{lemma:min} which shows that attributing a min-function using the origin as a reference point yields a uniform redistribution strategy.
\end{proof}

\subsection{Two-Cluster Case}

We observe that when there are only two clusters (the one on which the data point is assigned and the competitor, respectively denoted by $c$ and $k$) we get by application of Eq.\ \eqref{eq:mintakemost} that multiple terms are equal:
\begin{align}
R_k = h_k = f_c(\x)
\end{align}
We also recall that the rule we use for the first layer is given by
\input{equations/rule-directional}

Observing that the denominator of the propagation rule is equivalent to $h_k$, we get the closed form attribution
\begin{align}
R_i = (x_i - m_{ik}) \cdot w_{ik}
\label{eq:neon-relevance-twocluster}
\end{align}

\input{propositions/shapley-twoclusters}

This result naturally follows from application of Lemma \ref{lemma:linear} for the function $f_c(\x)$ and replacement value $\widetilde{\x} = \boldsymbol{m}_k$, and observing that the resulting Shapley value matches the output of NEON given in Eq.\ \eqref{eq:neon-relevance-twocluster}.

\section{Decision Function of Kernel K-Means}
\label{appendix:kernel-approximation}

We recall that to address the limitation of a simple discriminant built in terms of distances in kernel feature space, i.e.\
\begin{align}
\forall_{k \neq c}:~ \|\Phi(\x)&-\centroid_c\|^2 < \|\Phi(\x)-\centroid_k\|^2
\label{eq:kernel-decision}
\end{align}
we have proposed the alternate the discriminant:
\begin{align}
\forall_{k \neq c}:~ {\LME_{i \in \mathcal{C}_c}}^{-\gamma} &\big\{\|\x - \sv_i\|^2\big\} < {\LME_{j \in \mathcal{C}_k}}^{-\gamma} \big\{\|\x - \sv_j\|^2\big\}
\label{eq:kernel-decision-improved}
\end{align}
\input{propositions/kernel-approximation}

\begin{proof}
We inject the original squared distance
$$
d_c(\x) = \|\Phi(\x) - \centroid_c\|^2
$$
in the function $g_c$ and recall that the polylogarithm is given by $\mathrm{Li}_1(t) = - \log (1-t)$, a convex function. We arrive after a few steps of derivation to the function used in the second discriminant:
\begin{align*}
g_c(d_c(\x))
&= \frac{1}{\gamma} \mathrm{Li}_1 \Big(\frac{d_c(\x)}{2} + \Delta_c\Big) + \frac{1}{\gamma} H_c\\
&= - \frac{1}{\gamma} \log \Big(1-\frac{d_c(\x)}{2} - \Delta_c \Big) + \frac1\gamma \log \Big(\frac{|\mathcal{C}_c|}{Z_c}\Big)\\
&= - \frac1\gamma \log \big( \langle \Phi(\x), \centroid_c\rangle \big) + \frac1\gamma \log \Big(\frac{|\mathcal{C}_c|}{Z_c}\Big)\\
&= -\frac1\gamma \log \Big(\frac{Z_c}{|\mathcal{C}_c|} \frac{1}{Z_c}\sum_{i \in \mathcal{C}_c} \mathbb{K}(\x,\x_i)\Big)\\
&= -\frac1\gamma \log \Big(\frac{1}{|\mathcal{C}_c|}\sum_{i \in \mathcal{C}_c} \exp(-\gamma \|\x-\x_i\|^2)\Big)\\
&= {\LME_{i \in \mathcal{C}_c}}^{-\gamma} \big\{\|\x - \x_i\|^2\big\}
\end{align*}
\end{proof}

\section{Neuralization of Kernel K-Means}
\label{appendix:neuralization-kernel}

\input{propositions/kernel-neuralization}

\begin{proof}
First, we show that the $\LME^\gamma$ operator is commutative w.r.t. additive scalars:
\begin{align*}
{\LME_j}^\gamma\lbrace a_j\rbrace + c &= \frac1\gamma\log \frac1N \sum_j \exp(\gamma\cdot a_j) + c\\
&= \frac1\gamma \log \frac1N \sum_j\exp(\gamma\cdot(a_j+c))\\
&= {\LME_j}^\gamma\lbrace a_j + c\rbrace
\end{align*}
This allows for a more high level point of view that holds for hard- as well as soft-min pools: a difference of minima equals a minimax of differences,
\begin{align}
{\LME_j}^{-\gamma}\{a_j\} - {\LME_i}^{-\gamma}\{b_i\} = {\LME_j}^{-\gamma}\{{\LME_i}^{\gamma}\{a_j-b_i\}\}.
\end{align}
By exploiting this fact multiple times, we derive the following reformulation of the discriminant for kernel clustering. Let $d_{jk} = \|\x-\sv_j\|^2$.
\begin{align}
f_c &=  - {\LME_{i\in\mathcal C_c}}^{-\gamma}\lbrace d_{ic}\rbrace + \min_{k\neq c} \Big\{{\LME_{j\in\mathcal C_k}}^{-\gamma}\lbrace d_{jk}\rbrace\Big\}\\
&= \min_{k\neq c} \Big\{ {\LME}_{j\in\mathcal C_k}^{-\gamma}\lbrace d_{jk}\rbrace - {\LME_{i\in\mathcal C_c}}^{-\gamma}\lbrace d_{ic}\rbrace \Big\}\\
&= \min_{k\neq c}\Big\{{\LME}^{-\gamma}_{j\in\mathcal C_k}\big\lbrace {\LME_{i\in\mathcal C_c}}^{\gamma}\lbrace d_{jk} - d_{ic}\rbrace\big\rbrace\Big\}.
\end{align}
Finally, observing that $h_{ijk} = d_{jk} - d_{ic}$ completes the derivation.
\end{proof}

\section{Neuralization of Soft Clustering}
\label{appendix:neuralization-soft}

This section describes how to neuralize to soft k-means model, where the assignment onto clusters is given in a probabilistic manner via the softmax function:
\begin{align}
\quad p_c(\x) = \frac{1}{\mathcal{Z}}\exp(z_c(\x))
\label{eq:softmax}
\end{align}
where $z_c(\x)$ is the softmax logit for cluster $c$, and where $\mathcal{Z} = \sum_k \exp(z_k(\x))$ is a normalization term. We contribute two theoretical results (Lemmas \ref{lemma:relative} and \ref{lemma:absolute}) from which one can derive neural network equivalents for a number of practical soft clustering models. 

\smallskip

Consider first the task of explaining the decision of a soft clustering model in favor of a particular cluster $c$ rather than any other cluster, i.e.
\begin{align}
    \forall_{k \neq c}:~p_c(\x) > p_k(\x).
    \label{eq:decision-relative}
\end{align}

\begin{lemma}
\label{lemma:relative}
The decision function of Eq.\ \eqref{eq:decision-relative}
is equivalent to testing whether the log-likelihood ratio
\begin{align}
f_c(\x) = \log \Big( \frac{p_c(\x)}{\displaystyle \max_{k \neq c} p_k(\x)} \Big)
\label{eq:llratio-relative}
\end{align}
is positive. Furthermore, this log-likelihood ratio can be expressed in terms of the softmax logits as:
\begin{align}
f_c(\x) = \min_{k \neq c} \{z_c(\x) - z_k(\x)\}.
\label{eq:difflogits-relative}
\end{align}
\end{lemma}
\begin{proof} For the first part, we observe that the decision of Eq.\ \eqref{eq:decision-relative} can be equally expressed as $p_c(\x) > \max_{k \neq c} p_k(\x)$ and applying the logarithm gives us Eq.\ \eqref{eq:llratio-relative}. For the second part, we develop the log-likelihood ratio as:
\begin{align}
f_c(\x) &= \log \Big( \frac{p_c(\x)}{\displaystyle \max_{k \neq c} p_k(\x)} \Big) \nonumber\\
    &= \log p_c(\x) - \log (\max_{k \neq c} \{ p_k(\x)\}) \nonumber\\
    &= \log p_c(\x) - \max_{k \neq c} \{\log p_k(\x)\} \nonumber\\
    &= (z_c(\x) - \log \mathcal{Z}) - \max_{k \neq c} \{ z_k(\x) - \log \mathcal{Z}\} \nonumber\\
    &= z_c(\x) - \max_{k \neq c} \{z_k(\x)\} \nonumber\\
    &= \min_{k \neq c} \{z_c(\x) - z_k(\x)\},
\end{align}
which gives us the form of Eq.\ \eqref{eq:difflogits-relative}
\end{proof}

Consider now the decision whether the probability score in favor of a particular cluster $c$ is above some threshold $\theta$, regardless of the probability of cluster competitors, i.e.
\begin{align}
p_c(\x) > \theta.
    \label{eq:decision-absolute}
\end{align}

\begin{lemma}
\label{lemma:absolute}
The decision function of Eq.\ \eqref{eq:decision-absolute} is equivalent to testing whether the (shifted) log-likelihood ratio
\begin{align}
f_c(\x) &= \log \Big(\frac{p_c(\x)}{1-p_c(\x)}\Big) + \log \Big(\frac{1-\theta}{\theta}\Big)
\label{eq:llratio-absolute}
\end{align}
is positive. Furthermore, this log-likelihood ratio can be expressed in terms of the softmax logits as:
\begin{align}
f_c(\x) &= {\LME_{k \neq c}}^{-1}\Big\{ z_c(\x) -z_k(\x) - \log (N-1) + \log \Big(\frac{1-\theta}{\theta}\Big)\Big\}.
\label{eq:difflogits-absolute}
\end{align}
\end{lemma}

\begin{proof} For the first part, we observe that applying the exponential to Eq.\ \eqref{eq:llratio-absolute} gives $p_c(\x) \cdot (1-\theta) > (1-p_c(\x)) \cdot \theta$ which can then be simplified to Eq.\ \eqref{eq:decision-absolute}. For the second part, we develop the log-likelihood ratio as:
\begin{align*}
f_c(\x)
&= \log \Big(\frac{p_c(\x)}{1-p_c(\x)}\Big) + \log \Big(\frac{1-\theta}{\theta}\Big)\\
&= \log p_c(\x) - \log (1-p_c(\x)) + \log \Big(\frac{1-\theta}{\theta}\Big)\\
&= \log p_c(\x) - \log \Big(\sum_{k \neq c} p_k(\x)\Big) + \log \Big(\frac{1-\theta}{\theta}\Big)\\
&= \big(z_c(\x) - \log \mathcal{Z}\big) - \big(\log \sum_{k \neq c} \exp(z_k(\x)) - \log \mathcal{Z}\big) + \log \Big(\frac{1-\theta}{\theta}\Big)\\
&= z_c(\x) - \log \sum_{k \neq c} \exp(z_k(\x))  + \log \Big(\frac{1-\theta}{\theta}\Big)\\
&= - \log \sum_{k \neq c} \exp(-(z_c(\x)-z_k(\x)))  + \log \Big(\frac{1-\theta}{\theta}\Big)\\
&= - \log \frac{1}{N-1}\sum_{k \neq c} \exp(-(z_c(\x) -z_k(\x))) - \log(N-1)  + \log \Big(\frac{1-\theta}{\theta}\Big)\\
&= {\LME_{k \neq c}}^{-1}\big\{z_c(\x) -z_k(\x) \big\} - \log (N-1) + \log \Big(\frac{1-\theta}{\theta}\Big)\\
&= {\LME_{k \neq c}}^{-1}\Big\{ z_c(\x) -z_k(\x) - \log (N-1) + \log \Big(\frac{1-\theta}{\theta}\Big)\Big\},
\end{align*}
which gives us the form of Eq.\ \eqref{eq:difflogits-absolute}.
\end{proof}
The results provided by Lemmas \ref{lemma:relative} and \ref{lemma:absolute} will help us to derive neuralized forms for several practical soft clustering models, in particular, soft k-means, and a deep clustering model.

\subsection{Neuralization of Soft K-Means}
\label{appendix:soft-kmeans}

We consider a soft version of k-means where the probabilities are generated using the softmax function of Eq.\ \eqref{eq:softmax} and where the logits entering into the softmax function are (rescaled) square distances:
\begin{align}
z_k(\x) = -\tau \|\x-\centroid_k\|^2.
\label{eq:logits-softkmeans}
\end{align}
The parameter $\tau$ is a scaling parameter, commonly referred as `stiffness'. Applying Lemmas \ref{lemma:relative} and \ref{lemma:absolute}, and observing that a difference of logits can be written as a linear function of $\x$, i.e.,
\begin{align*}
    z_c(\x) - z_k(\x) &= -\tau \|\x-\centroid_c\|^2 + \tau \|\x-\centroid_k\|^2\\[1mm]
    &= 2\tau \cdot \x^\top (\centroid_c - \centroid_k) + \tau \cdot (\|\centroid_k\|^2 - \|\centroid_c\|^2)
\end{align*}
we can reproduce the decision functions of Eq.\ \eqref{eq:decision-relative} by the neural network:
\begin{boxnetwork}[Neuralized soft k-means (relative)]
\begin{align*}
h_k &= \w_k^\top \x + b_k & \text{(layer 1)}\\
f_c &= \min_{k \neq c}\{h_k\} & \text{(layer 2)}
\end{align*}
\end{boxnetwork}
where $\w_k = 2 \tau \cdot (\centroid_c - \centroid_k)$ and $b_k = \tau \cdot (\|\centroid_k\|^2 - \|\centroid_c\|^2)$, and testing for $f_c \geq 0$. Likewise, we can reproduce the decision function of Eq. \eqref{eq:decision-absolute} by the neural network:
\begin{boxnetwork}[Neuralized soft k-means (absolute)]
\begin{align*}
h_k &= \w_k^\top \x + b_k & \text{(layer 1)}\\
f_c &= {\LME_{k \neq c}}^{-1}\{h_k\} & \text{(layer 2)}
\end{align*}
\end{boxnetwork}
where $\w_k = 2\tau \cdot (\centroid_c - \centroid_k)$ and $b_k = \tau \cdot (\|\centroid_k\|^2 - \|\centroid_c\|^2) - \log(N-1) + \log ((1-\theta)/\theta)$, and testing for $f_c > 0$.

\subsection{Neuralization of Deep Soft Clustering}
\label{appendix:soft-deep}

We recall that the decision function implemented by deep soft clustering (cf.\ Section IV of the main paper) is given by:
\input{equations/softdeep-decision}
\input{propositions/softdeep-neuralization}
\begin{proof}
The proof follows from observing that the decision function is of the same type as Eq.\ \eqref{eq:softmax} with logit $z_c(\x) = \centroid_c^\top \ba$, applying Lemma \eqref{lemma:relative}, and observing that the difference of logits simplifies to $z_c(\x) - z_k(\x) = (\centroid_c-\centroid_k)^\top \ba$, i.e.\ a homogeneous linear model built on the activation vector $\ba$.
\end{proof}

We recall that the decision function implemented by deep soft clustering, when considering an absolute probability threshold (cf.\ Section IV of the main paper), is given by:
\input{equations/softdeep-decision-2}
where $p_c(\x)$ is defined in the same way as in Eq.\ \eqref{eq:softdeep-decision}.
\input{propositions/softdeep-neuralization-2}
\begin{proof}
The proof proceeds in a similar way as for Proposition \ref{proposition:softdeep-neuralization}, but making use of Lemma \ref{lemma:absolute} instead of Lemma \ref{lemma:relative}.
\end{proof}

\section{Training Algorithm for Kernel K-Means}
\label{appendix:training}

We consider an equal-weight mixture of tied-isotropic Gaussians for each cluster, i.e.\ membership to a cluster is related to the following likelihood:
\begin{align}
    p_k(\x) = \sum_{j=1}^M\frac1M\left(\frac\gamma\pi\right)^{\frac{d}2}\exp(-\gamma\|\x - \sv_j\|^2)
\end{align}
Here, $\x\in\mathbb{R}^d$ and $M$ is the number of components that represent cluster $k$. We pick the same number of components for each cluster, hence the index is omitted. The negative log-likelihood takes the form 
\begin{align}
    -\log p_k(\x) = \gamma{\LME_{j\in{\cal C}_k}}^{-\gamma}\lbrace\|\x-\sv_j\|^2\rbrace - \frac{d}2\log\frac\gamma\pi.
\end{align}
Let $(\x_n)_{n=1}^N$ be our dataset. We learn the cluster assignment $\delta_{nk}$, the support vectors $\sv_j$, and the scale parameter $\gamma$ to minimize the objective
\begin{align}
{\cal L}\left((\sv_j)_j, \gamma, (\delta_{nk})_{nk}\right) = \sum_k \sum_{n} \delta_{nk} \gamma {\LME_{j \in \mathcal{C}_k}}^{-\gamma} \{ \|\x_n-\sv_j \|^2 \} - \frac{Nd}{2}\log\gamma \label{eq:nll_kernel}
\end{align}
where $\delta_{nk}$ is an indicator function for the membership of data point $n$ to cluster $k$. We apply an EM-style procedure, which alternates the (hard) cluster assignment (to the mixture $p_k$ of largest likelihood) and the computation of centroids/support vectors and scale parameter $\gamma$. The update rules are
\begin{align}
    \sv_j &\leftarrow \sum_n \frac{{\mathbb K}_{nj}}{\sum_{n}{\mathbb K}_{nj}} \x_n \\
    \gamma &\leftarrow \Big(\frac{2}{Nd}\sum_n\sum_k\sum_{j\in{\cal C}_k} {\mathbb K}_{nj}\cdot \|\x_n - \sv_j\|^2\Big)^{-1}
\end{align}
with ${\mathbb K}_{nj} = \delta_{nk}\cdot\frac{\exp(-\gamma\|\x_n - \sv_j\|^2)}{\sum_{j\in{\cal C}_k}\exp(-\gamma\|\x_n - \sv_j\|^2)}$, a softmax.
To avoid singular clusters, we add a small value $\varepsilon = 10^{-9}$ to the rhs of the $\gamma$ update rule before taking the inverse. We also add a tiny amount of Gaussian noise to all support vectors before the E-step. This helps avoiding repeated support vectors. As a stopping criterion, we fix the number of iterations to 100. In order to avoid bad local optima, we start the whole procedure 10 times, and pick the solution with smallest value of ${\cal L}$ in Eq. (\ref{eq:nll_kernel}).

\section{KDE-Based Imputation}
\label{appendix:imputation}

For our prediction difference analysis (PDA) explanation baseline, as well as in our AUC evaluation procedure, we need a mechanism to impute missing features. We choose to replace missing features by sampling from the conditional distribution of a kernel density estimation (KDE) model. The KDE model is learned to approximate the data. Let $(\x_n)_{n=1}^N$ be the whole training set. The KDE model is defined as:
\begin{align}
p(\x) = \frac1N \sum_n {\cal N}(\x\mid\x_n, \sigma^2I)
\label{eq:kde}
\end{align}
The single parameter $\sigma$ is estimated via a leave-one-out procedure: The leave-one-out likelihood simply removes one term from the sum in Eq.\ \eqref{eq:kde}:
\begin{align}
    p_{-n}(\x) = \frac{1}{N-1}\sum_{n' \neq n}
    {\cal N}(\x\mid\x_{n'}, \sigma^2I)
\end{align}
Then, we minimize
\begin{align}
    {\cal L}(\gamma) = \sum_n -\log p_{-n}(\x_n).
\end{align}
This is achieved by applying the iteration:
\begin{align}
    \sigma^2 \leftarrow \frac1{Nd} \sum_n\sum_{n'\neq n} \frac{\exp\left(-\frac{\|\x_n -
\x_{n'}\|^2}{2\sigma^2_{\mathrm{old}}}\right)}{\sum_{n'\neq n}\exp\left(-\frac{\|\x_n - \x_{n'}\|^2}{2\sigma^2_{\mathrm{old}}}\right)}\|
\x_n-\x_{n'}\|^2
\end{align}
until convergence. An advantage of the KDE model is that we can easily access conditional probabilities of the model, which is useful for imputation. Let ${\cal F}$ be the set indices that must be imputed and let ${\cal P}$ be those that are given. The conditional distribution $p(\x_{\cal F}\mid\x_{\cal P})$, which we use for imputation, is given in closed form as:
\begin{align}
    p(\x_{\cal F}\mid\x_{\cal P}) &= \sum_n \alpha_n 
    {\cal N}(\x_{\cal F}\mid [\x_n]_{\cal F}, \sigma^2I)
    \intertext{where}
    \alpha_n &= \frac{\exp\left(-\frac{\|\x_{\cal P} - [\x_n]_{{\cal P}}\|^2}{2\sigma^2}\right)}{\sum_{n'} \exp\left(-\frac{\|\x_{\cal P} - [\x_{n'}]_{{\cal P}}\|^2}{2\sigma^2}\right)}
\end{align}
To sample from the conditional distribution, we first sample $n\sim \mathrm{Cat}((\alpha_n)_n)$, and then $\x_{\cal F} \sim {\cal N}(\x_{\cal F}\mid [\x_n]_{\cal F}, \sigma^2I)$. 

\section{Datasets}
\label{appendix:datasets}

Datasets were selected from the UCI repository by the following joint criteria: (1) dataset appears in category ``clustering'', (2) text, time-series, and sequential datasets are excluded, (3) dataset has 5 to 70 attributes and 100 to 2000 instances, (4) attributes are mostly real-valued. Then, the following pre-processing is performed for each dataset: First, binary and categorical attributes (such as labels) are removed. Then, missing values are replaced by the mean of the attribute. Finally, data is normalized to mean zero and standard deviation 1 along each dimension. We also consider several non-UCI datasets, in particular the 20Newsgroup text dataset and the STL-10 images dataset. The list of datasets we consider and the link where they can be found is given in Table \ref{table:datasets}.
\begin{table}[t]
\caption{List of datasets used in the experiments along with their urls.}
\label{table:datasets}
\centering
\begin{tabular}{ll}\toprule
Dataset & URL \\\midrule
BuddyMove Data Set ({\tt buddy}) & \url{https://archive.ics.uci.edu/ml/datasets/BuddyMove+Data+Set} \\
Census ({\tt c2000}) & \url{http://cs.joensuu.fi/sipu/datasets/}\\
HCV data ({\tt hepac}) & \url{https://archive.ics.uci.edu/ml/datasets/HCV+data} \\
20Newsgroup ({\tt news}) & \url{http://qwone.com/~jason/20Newsgroups/}\\
Sales Transactions Dataset Weekly ({\tt sales}) & \url{https://archive.ics.uci.edu/ml/datasets/Sales_Transactions_Dataset_Weekly} \\
Seeds (\texttt{seeds}) & \url{https://archive.ics.uci.edu/ml/datasets/seeds} \\
STL-10 ({\tt STL-10}) & \url{https://cs.stanford.edu/~acoates/stl10}\\
Travel Reviews (\texttt{trpad}) & \url{https://archive.ics.uci.edu/ml/datasets/Travel+Reviews} \\
Water Treatment Plant (\texttt{water}) & \url{https://archive.ics.uci.edu/ml/datasets/water+treatment+plant}\\
Wholesale customers (\texttt{whlsl}) & \url{https://archive.ics.uci.edu/ml/datasets/wholesale+customers} \\
Wine ({\tt winer}) & \url{https://archive.ics.uci.edu/ml/datasets/wine} \\
\bottomrule
\end{tabular}
\end{table}

\section{Additional Evaluation of Runtime Performance}
\label{appendix:runtime}

Figure \ref{fig:time_vs_KD} shows the runtime of computing explanations for the whole {\tt winer} dataset. We used the Python function {\tt time.process\_time\_ns} to measure runtime. IG-10 has ten times the runtime of sensitivity analysis. PDA runtime heavily depends on the replacement-strategy: For a sampling-based replacement value, the runtime grows much faster for larger dimensions than a fixed replacement value. NCA, NEON, sensitivity analysis and $\x^2$, grow linearly at a negligible slope. The number of clusters has limited impact on runtime. Deviations from our theoretical runtime analysis in Table 2 in the main text can be mainly attributed to side computations and to hardware optimization, such as cache optimization.
\begin{figure}[h!]
    \centering
    \includegraphics[width=.65\linewidth]{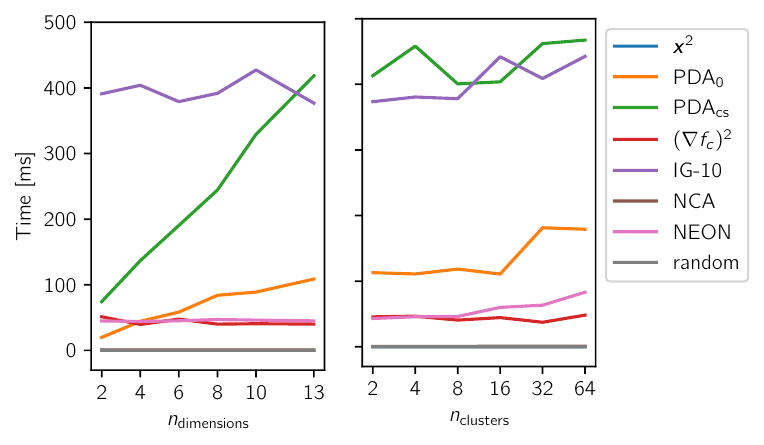}
    \caption{Runtime of explaining the predictions of a k-means model on the  {\tt winer} dataset, as a function of the number of retained input dimensions and the number of clusters}.
    \label{fig:time_vs_KD}
\end{figure}

\section{Additional Results for the VGG-16 Network}
\label{appendix:vgg16}

This appendix gives additional details and intermediate results for the quantitative experiment of Section VI-C in the main paper. We consider images from the PASCAL\,VOC\,2007 dataset \cite{pascal-voc-2007} along with their segmentations masks. For each image, we add a `background' segment representing all non-segmented areas. For a selection of images, we compute the heatmaps summaries obtained by applying NEON or one of the three other methods in our benchmark (FM, LO and NetDissect \cite{netdissect2017}) at a given layer of the VGG-16 network \cite{simonyan_very_2015}.

Figure \ref{app:N17} shows best, median and worst case images as evaluated by our heatmap-segmentation matching metric at the output of block 5. Images from the dataset are ranked based on their matching scores averaged over NEON, FM, LO and NetDissect. We superimpose them with their matched segmentation mask displayed as a black contour. The `background' segment is displayed with a solid border frame. The scores in the bottom right of each heatmap are cosine similarities between the heatmap and the matching segmentation mask.

\begin{figure*}[h]
\centering
\includegraphics[width=.9\textwidth]{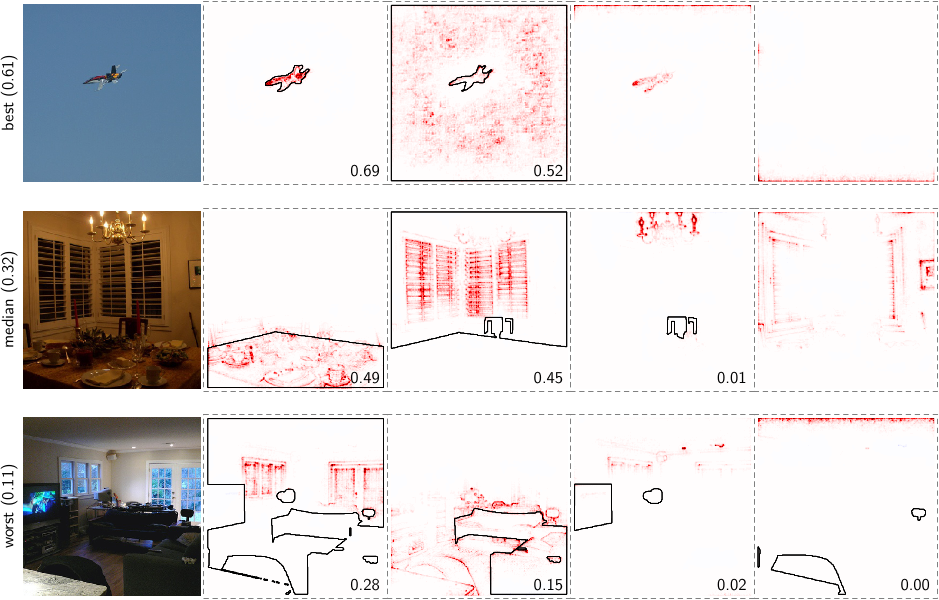}
\caption{NEON of a k-means model built at the output of block 5 of the VGG-16 model, and applied to images with best\,/\,median\,/\,worst matching between heatmaps and segmentations.}\label{app:N17}
\end{figure*}

We observe that the best case image depicts a simple scene composed of clearly distinguishable objects with different colors and textures. Normally, objects that appear several times form a cluster, although sometimes there is no specific segmentation for that kind of object, e.g. windows or candles in the middle row. On the other hand, there are also segments for background objects that do not form their own cluster, such as the chair. We can also observe that even for the worst case example, heatmaps may still focus on distinct objects, e.g. windows or table clutter.

\medskip

Figure \ref{app:M17} shows heatmap summaries at the output of block 5 for NEON and the LO, FM, and NetDissect methods, on some image with typical matching quality.

\begin{figure*}[h]
\centering
\includegraphics[width=.9\textwidth]{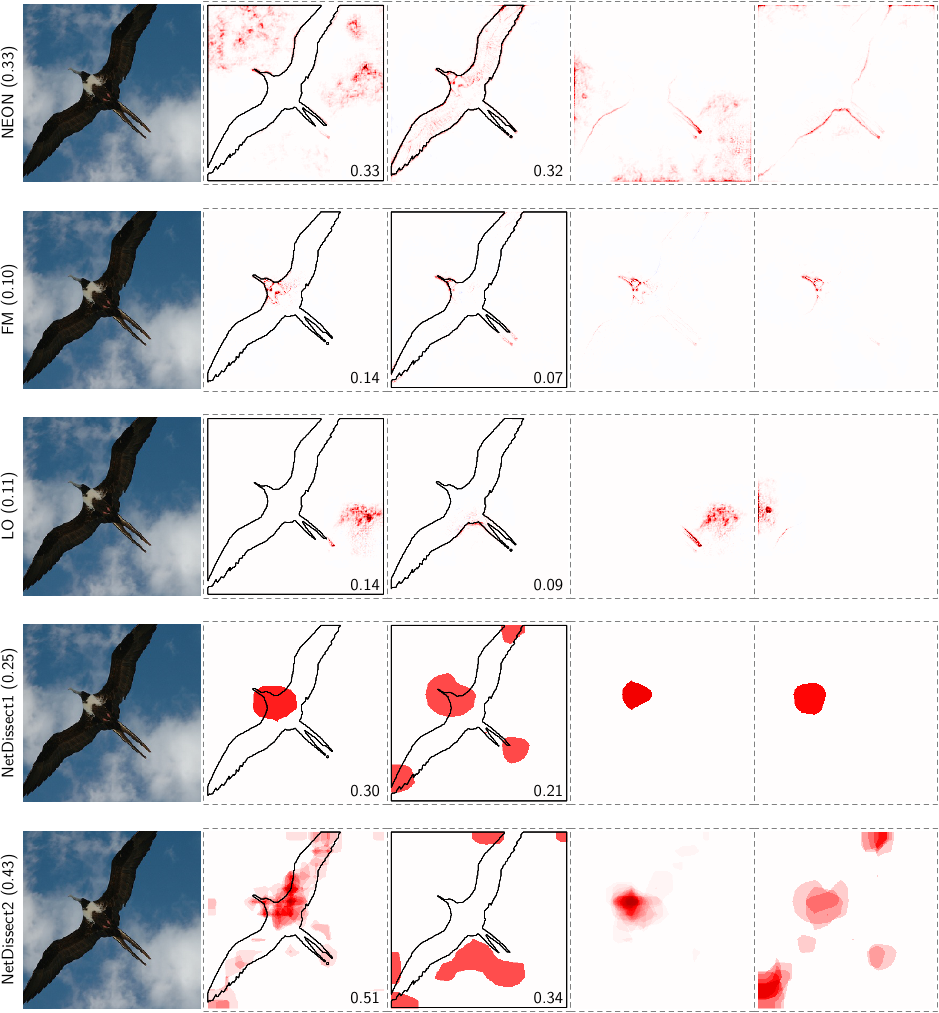}
\caption{NEON compared to the FM, LO and NetDissect baselines, when considering a model built at the output of block 5 of the VGG-16 model. We show an image corresponding to a median matching quality between heatmaps and segmentation masks.}
\label{app:M17}
\end{figure*}

We observe for this image that the heatmaps produced by FM focus multiple times on the same region of the input image, thereby not delivering an appropriate spatial summary. The LO heatmaps are too localized to exhaustively capture large image parts (e.g.\ the background). Similarly to FM, the NetDissect1 method (top-$4$ concepts) is affected by a redundancy problem where the different concepts (e.g. texture, color, object) are bound to the same image regions. In the NetDissect2 variant, where concepts are grouped into $4$ clusters, the summary becomes more complete, leading to a higher cosine similarity. Finally, our proposed method NEON, although not making use of any supervised information besides what is already contained in the feature representation, produces qualitatively the most satisfying summary. The cosine similarity is here mainly limited by the heatmap sparsity that is especially strong at the output of block 5. Sparsity prevents a full correlation with the dense segmentation masks. While we have used the raw NEON output in our comparison, further benchmark-specific post-processing steps, e.g.\ spatial interpolation, could in principle be used to further improve the score.

\bibliographystyle{IEEEtran}
\bibliography{paper}

\end{document}
